# Supplementary material for: Revealing charge-tunneling processes between a quantum dot and a superconducting island through gate sensing
Source: arXiv:1903.09066 ancillary file (2019-10-18)
Supplement: Supplementary file 1 [file Supplement.pdf]

# Revealing charge-tunneling processes between a quantum dot and a superconducting island through gate sensing

Jasper van Veen,<sup>1</sup> Damaz de Jong,<sup>1</sup> Lin Han,<sup>1</sup> Christian Prosko,<sup>1</sup> Peter Krogstrup,<sup>2</sup> John D. Watson,<sup>3</sup> Leo P. Kouwenhoven,<sup>1,3</sup> and Wolfgang Pfaff<sup>3,\*</sup>

<sup>1</sup>*QuTech and Kavli Institute of Nanoscience,  
Delft University of Technology, 2600 GA Delft, The Netherlands*

<sup>2</sup>*Center for Quantum Devices, Niels Bohr Institute,  
University of Copenhagen & Microsoft Quantum Materials Lab Copenhagen, Denmark*

<sup>3</sup>*Microsoft Quantum Lab Delft, Delft University of Technology, 2600 GA Delft, The Netherlands*  
(Dated: October 18, 2019)

## I. RESONATOR CHARACTERIZATION

In this section, we present the frequency response for both resonators (Fig. S1a,b). From fits to the asymmetric resonator model described in section II (with  $\Omega \rightarrow \infty$  i.e. in Coulomb blockade), we extract the resonance frequency  $f_0$  and the loaded quality factor  $Q = f_0/\kappa$ . The resonance frequency is set by the inductance of an off-chip, superconducting spiral inductor ( $L = 420$  nH), and the parasitic capacitance of the resonator to its environment [1].

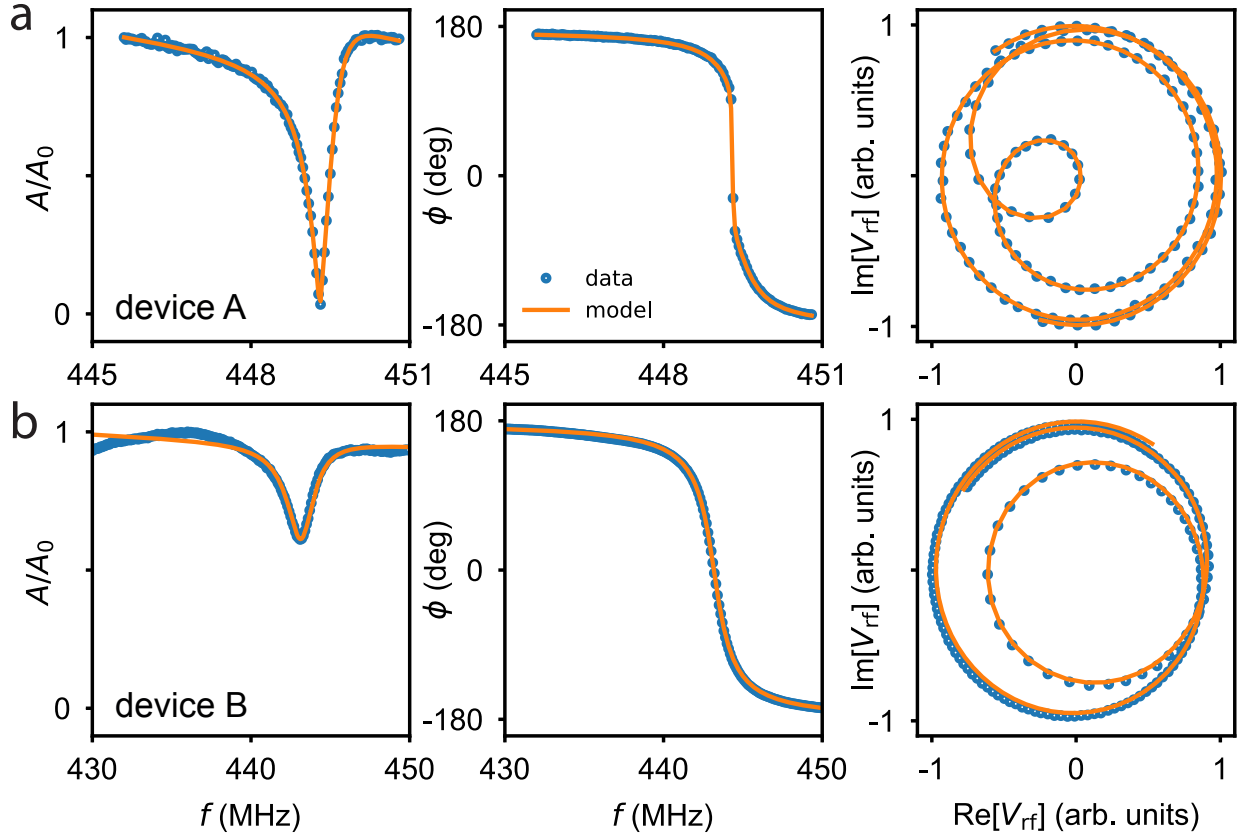

FIG. S1: **Resonator characterization.** The resonators are characterized by measuring their response  $V_{\text{rf}} = Ae^{i\phi}$  versus frequency across their resonance frequency. The left panels show the (normalized) amplitude  $A/A_0$  response; the middle panels the phase response  $\phi$  (corrected for the electrical delay in our setup); and the right panels the (normalized) real versus the imaginary part of the response. **a)** For device A, we find  $f_0 = 449.4$  MHz and  $Q = 620$ . **b)** For device B, we find  $f_0 = 443.2$  MHz and  $Q = 194$ .

## II. MODEL FOR THE RESONATOR RESPONSE

In this section, we present the model used to fit the linecuts in Fig. 2 of the main text. We solve the Heisenberg-Langevin equations for the reflected probe field of a resonator coupled to a double quantum dot [2]. In order to match our data, we add a phenomenological, complex scattering parameter ( $S$ ) to account for impedance mismatches in our setup, following the reasoning presented in Ref. 3. Combined, we arrive at

$$\frac{a_{\text{out}}}{a_{\text{in}}} = \frac{\kappa_{\text{ext}}}{i\Delta_0 + \kappa/2 + g_{\text{eff}}\chi} - 1 + |S|e^{i\phi}, \quad (\text{S1})$$

with susceptibility

$$\chi = \frac{g_{\text{eff}}}{-\Delta + i\gamma/2}. \quad (\text{S2})$$

In these equations,  $a$  is the probe field,  $\Delta_0 = \omega_0 - \omega$  the detuning between the resonator and the probe field;  $\Delta = \Omega/\hbar - \omega$  the detuning between the double dot and the probe field, where  $\Omega = \sqrt{4t_C^2 + \epsilon^2}$  with  $t_C$  the tunnel coupling and  $\epsilon$  the detuning between the quantum dots;  $\kappa_{\text{ext}}$  the external coupling rate;  $\kappa = \kappa_{\text{ext}} + \kappa_{\text{int}}$  the total loss rate with  $\kappa_{\text{int}}$  the internal loss rate;  $g_{\text{eff}} = g_0 \frac{2t_C}{\Omega}$  the coupling between the resonator and double dot; and  $\gamma$  the dephasing rate of the double dot.

TABLE S1: Overview of the parameters used to fit the resonator response in Fig. 2c. of the main text.

| parameter              | value             |
|------------------------|-------------------|
| $\kappa_{\text{ext}}$  | 0.41 MHz          |
| $\kappa$               | 0.73 MHz          |
| $t_C^{\text{even}}$    | 20 GHz            |
| $g_0$                  | 100 MHz           |
| $\gamma^{\text{even}}$ | 2.6 GHz           |
| $\gamma^{\text{odd}}$  | 1.0 GHz           |
| $S$                    | $-0.054 - i0.354$ |

### III. ADDITIONAL COULOMB DIAMOND MEASUREMENTS

In this section, we present additional Coulomb blockade measurements of the quantum dot (QD) in Fig. S2, and the superconducting island (SC) of device A in Fig. S3.

From the Coulomb diamonds in Fig. S2, we extract the QD charging energy and estimate the typical level spacing of the dot. We find that the charging energy is the largest energy scale for both QD-SC systems. Moreover, the level spacing,  $\delta$ , exceeds the thermal energy for both QDs, and it fluctuates with the charge occupation in the QD.

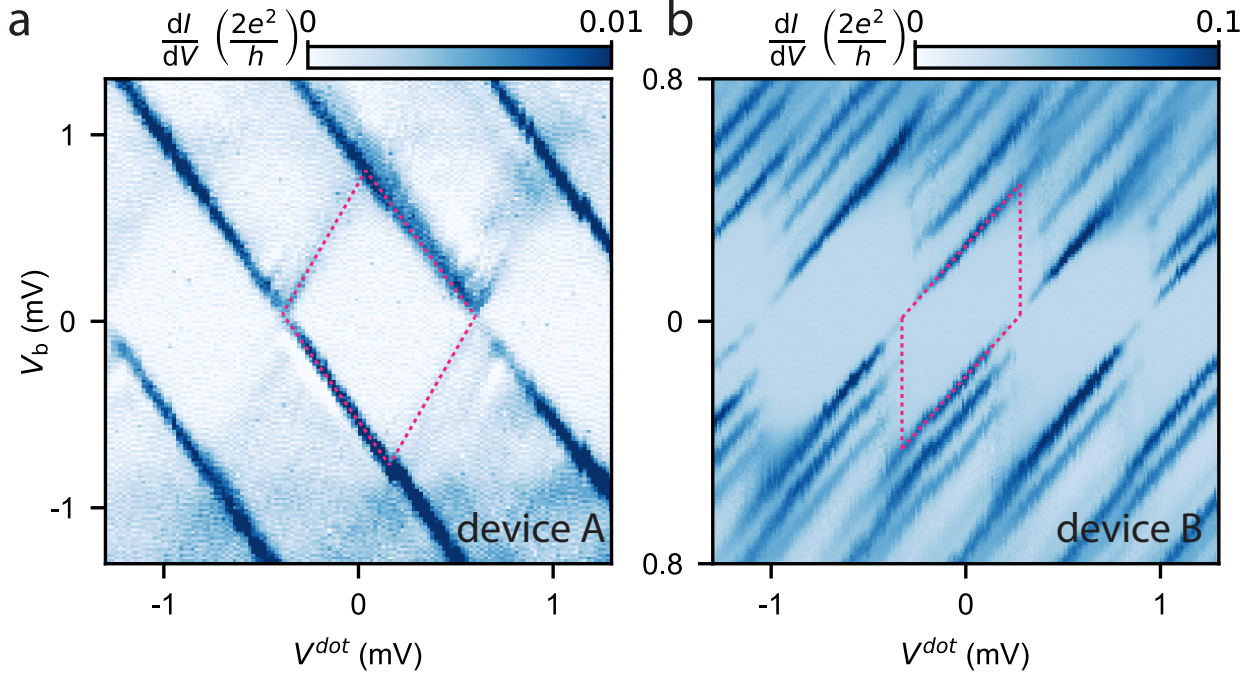

FIG. S2: **Coulomb blockade measurements on the quantum dots.** **a)** For device A, the conductance is calculated from the numerical derivative of the measured current. We extract  $E_C^{\text{QD}} \approx 300 \mu\text{eV}$ ,  $\delta = 50 - 150 \mu\text{eV}$ , and  $\alpha^{\text{QD}} = 0.8$ . **b)** For device B, we obtain  $E_C^{\text{QD}} \approx 200 \mu\text{eV}$ ,  $\delta = 100 - 170 \mu\text{eV}$ , and  $\alpha^{\text{QD}} = 0.72$ . The pink-dashed lines serve as guide to the eye to indicate a single Coulomb diamond.

Figure S3 shows Coulomb diamonds for the SC of device A obtained via current measurements at the same gate settings as the diamond scan shown in Fig. 1b of the main text. The data is presented in the main text is measured using RF reflectometry from the source of the QD-SC system. The conductance shown here drops back to zero when  $V_b$  increase above the height of the small odd diamond. This indicates that for the odd charge states the current is carried by a discrete, subgap state. In contrast, if the current is carried by a continuum of states, the conductance would remain constant.

### IV. ADDITIONAL CHARGE STABILITY DIAGRAMS DEVICE A

In this section, we present additional CSDs of the hybrid double dot in device A measured via the resonator connected to the plunger gate of the superconducting island (circuit not shown in Fig. 1) (Fig. S4). This data is measured simultaneously with the data presented in Fig. 2 of the main text, and is used to determine the location of the SC-lead transitions (pink dashed lines in Fig. 2).

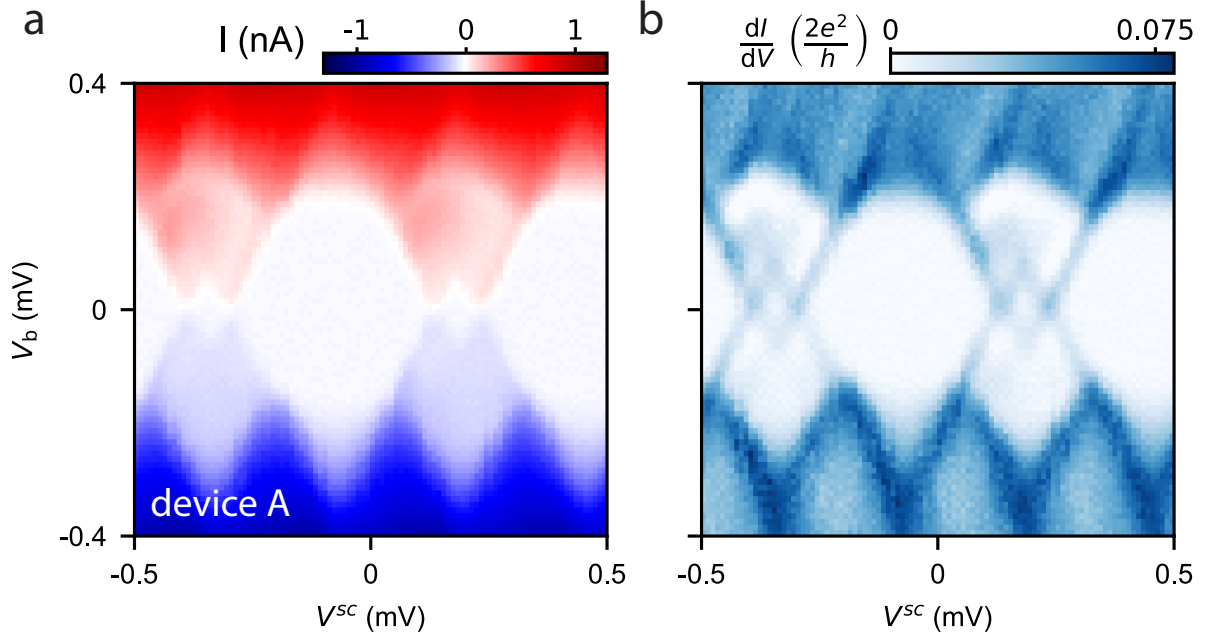

FIG. S3: Coulomb blockade measurements of the superconducting island in device A. Left panel: current data, right panel: differential conductance obtained by taking the numerical derivative of the current data.

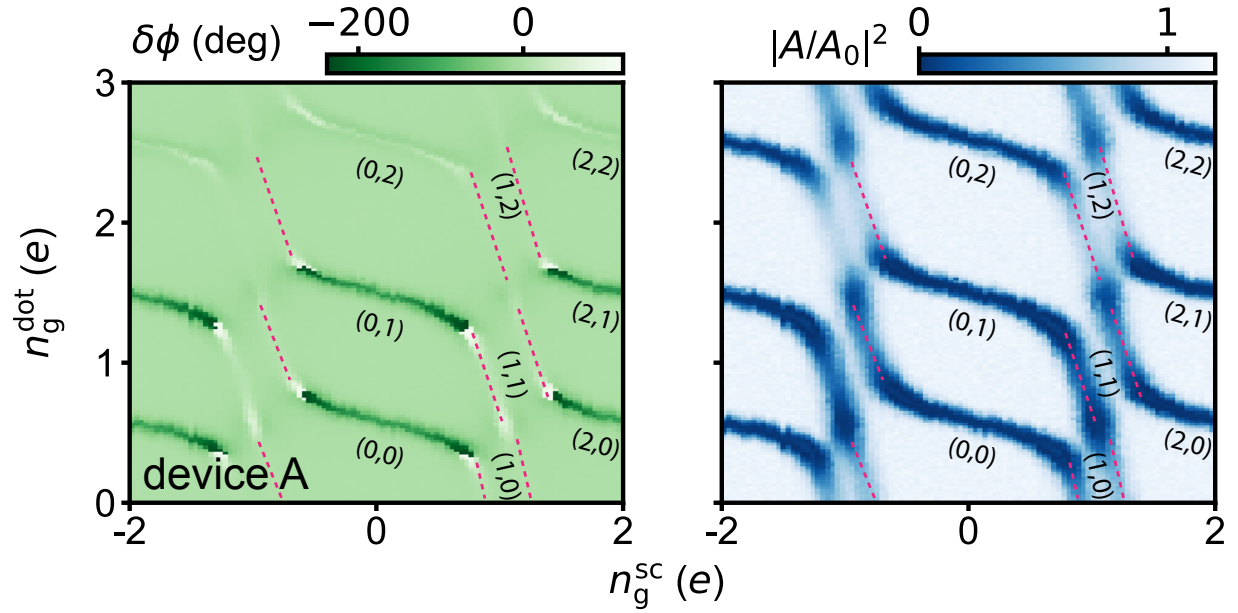

FIG. S4: Charge stability diagram measured with gate-sensing via the plunger gate of the SC. Left: phase, right: amplitude. The pink-dashed lines indicate, as guides to the eye, the SC-lead transitions.

## V. SIMULATION OF THE CHARGE STABILITY DIAGRAMS

In this section, we discuss the phenomenological model used to simulate the charge stability diagrams shown in Fig. 3 of the main text. We start with the Hamiltonian of the QD-SC system

$$\hat{H} = \hat{H}_C + \hat{H}_{\text{BCS}} + \hat{H}_T, \quad (\text{S3})$$

where  $\hat{H}_C$  describes the charging energy of the combined system,  $\hat{H}_{\text{BCS}}$  the superconductivity on the island and the induced superconductivity in the dot, and  $\hat{H}_T$  the coupling between the two systems. Note that we neglect the level spacing in both systems. For the superconducting island, this is justified since its estimated level spacing is on the order of several mK. However, for the QD, where  $\delta \approx 100 \mu\text{eV}$ , this is a large simplification. We model the charging term by  $\hat{H}_C = \hat{H}_C^{\text{QD}} + \hat{H}_C^{\text{SC}} + \hat{H}_{C_m}$

$$\hat{H}_C^i = \sum_{n^i} E_C^i (n^i - n_g^i)^2 \quad (\text{S4})$$

$$\hat{H}_{C_m} = \sum_{n^{\text{SC}}, n^{\text{QD}}} E_{C_m} (n^{\text{SC}} - n_g^{\text{SC}}) (n^{\text{QD}} - n_g^{\text{QD}}) \quad (\text{S5})$$

where  $i = \text{QD}, \text{SC}$  labels the system;  $E_C^i$  is the charging energy,  $n_g^i$  the gate charge, and  $n^i$  labels the charge state.

We approximate the BCS Hamiltonian by assuming that only the lowest single particle state with energy  $E_0$  is relevant

$$\hat{H}_{\text{BCS}} \approx \begin{cases} 0 & n^i \text{ is even} \\ E_0^i & n^i \text{ is odd.} \end{cases} \quad (\text{S6})$$

Note that  $E_0 = \Delta$  in case there are no subgap states present on the SC. Usually,  $E_0^{\text{QD}} = 0$ , we included this term to be able to model induced superconducting correlations in the quantum dot when the QD-SC coupling is strong.

Lastly, for the tunneling Hamiltonian, we include both  $1e$  and  $2e$  charge-transfer processes:  $\hat{H}_T = \hat{H}_T^{1e} + \hat{H}_T^{2e}$  with

$$\hat{H}_T^{1e} = \sum_{n^{\text{SC}}, n^{\text{QD}}} t_{1e} |n^{\text{SC}} - 1\rangle \langle n^{\text{QD}} + 1| + \text{h.c.} \quad (\text{S7})$$

$$\hat{H}_T^{2e} = \sum_{n^{\text{SC}}, n^{\text{QD}}} t_{2e} |n^{\text{SC}} - 2\rangle \langle n^{\text{QD}} + 2| + \text{h.c.}, \quad (\text{S8})$$

where  $t_{1e}$  ( $t_{2e}$ ) is the tunneling amplitude for the  $1e$  ( $2e$ ) process.

To simulate the charge stability diagrams, we construct a Hamiltonian based of a finite number of charge states  $|n^{\text{SC}}, n^{\text{QD}}\rangle = |-4, -4\rangle, |-4, -3\rangle, \dots, |4, 4\rangle$ , using Kwant [4], and numerically solve for its eigenvalues and eigenvectors. We use the eigenvectors to calculate the charge expectation value of the total system which we compare to the data.

### A. Additional information simulations

TABLE S2: Overview of the parameters used in the simulations.

| Simulation | $E_C^{\text{SC}} (\mu\text{eV})$ | $E_C^{\text{QD}} (\mu\text{eV})$ | $E_{C_m} (\mu\text{eV})$ | $E_0^{\text{SC}} (\mu\text{eV})$ | $E_0^{\text{dot}} (\mu\text{eV})$ | $t_{1e} (\mu\text{eV})$ | $t_{2e} (\mu\text{eV})$ |
|------------|----------------------------------|----------------------------------|--------------------------|----------------------------------|-----------------------------------|-------------------------|-------------------------|
| Fig 3a     | 72                               | 230                              | 50                       | 88                               | 0                                 | 9                       | 0                       |
| Fig 3c     | 72                               | 230                              | 60                       | 88                               | 18                                | 176                     | 308                     |
| Fig S5     | 112                              | 500                              | 50                       | 72                               | 0                                 | 35                      | 0                       |

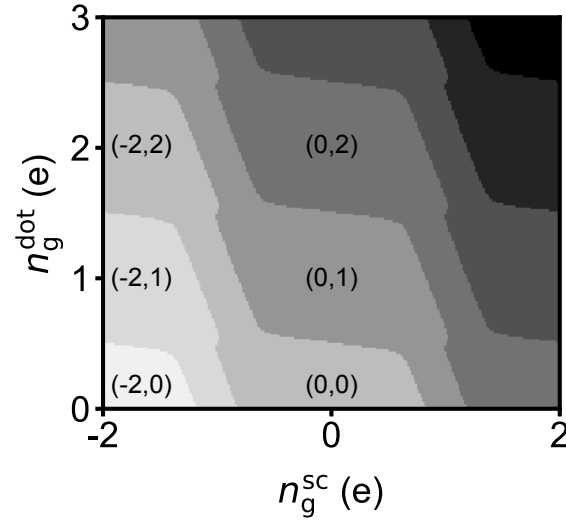

FIG. S5: **Simulation of the charge stability diagram of Fig 2. of the main text.** The gray scale indicates the sum of the charge in the hybrid double dot.

---

\* wolfgang.pfaff@microsoft.com

- [1] J. M. Hornibrook, J. I. Colless, A. C. Mahoney, X. G. Croot, S. Blanvillain, H. Lu, A. C. Gossard, and D. J. Reilly, *Frequency multiplexing for readout of spin qubits*, Applied Physics Letters **104**, 103108 (2014).
- [2] K. D. Petersson, L. W. McFaul, M. D. Schroer, M. Jung, J. M. Taylor, A. A. Houck, and J. R. Petta, *Circuit quantum electrodynamics with a spin qubit*, Nature **490**, 380 (2012).
- [3] M. S. Khalil, M. J..A. Stoutimore, F. C. Wellstood, and K. D. Osborn, *An analysis method for asymmetric resonator transmission applied to superconducting devices*, Journal of Applied Physics **111**, 054510 (2012).
- [4] C. W. Groth, M. Wimmer, A. R. Akhmerov, and X. Waintal, *Kwant: a software package for quantum transport*, New Journal of Physics **16**, 063065 (2014).
